# Supplementary material for: Critic-Guided Decoding for Controlled Text Generation
Source: arXiv:2212.10938 source file (2022-12-21)
Supplement: Supplementary file 1 [file Appendix.tex]

\section{Effect of size of the CriticControl subset}
\label{sec:appendix A}

\begin{figure}[ht!]
\centering
\includegraphics[width=\columnwidth]{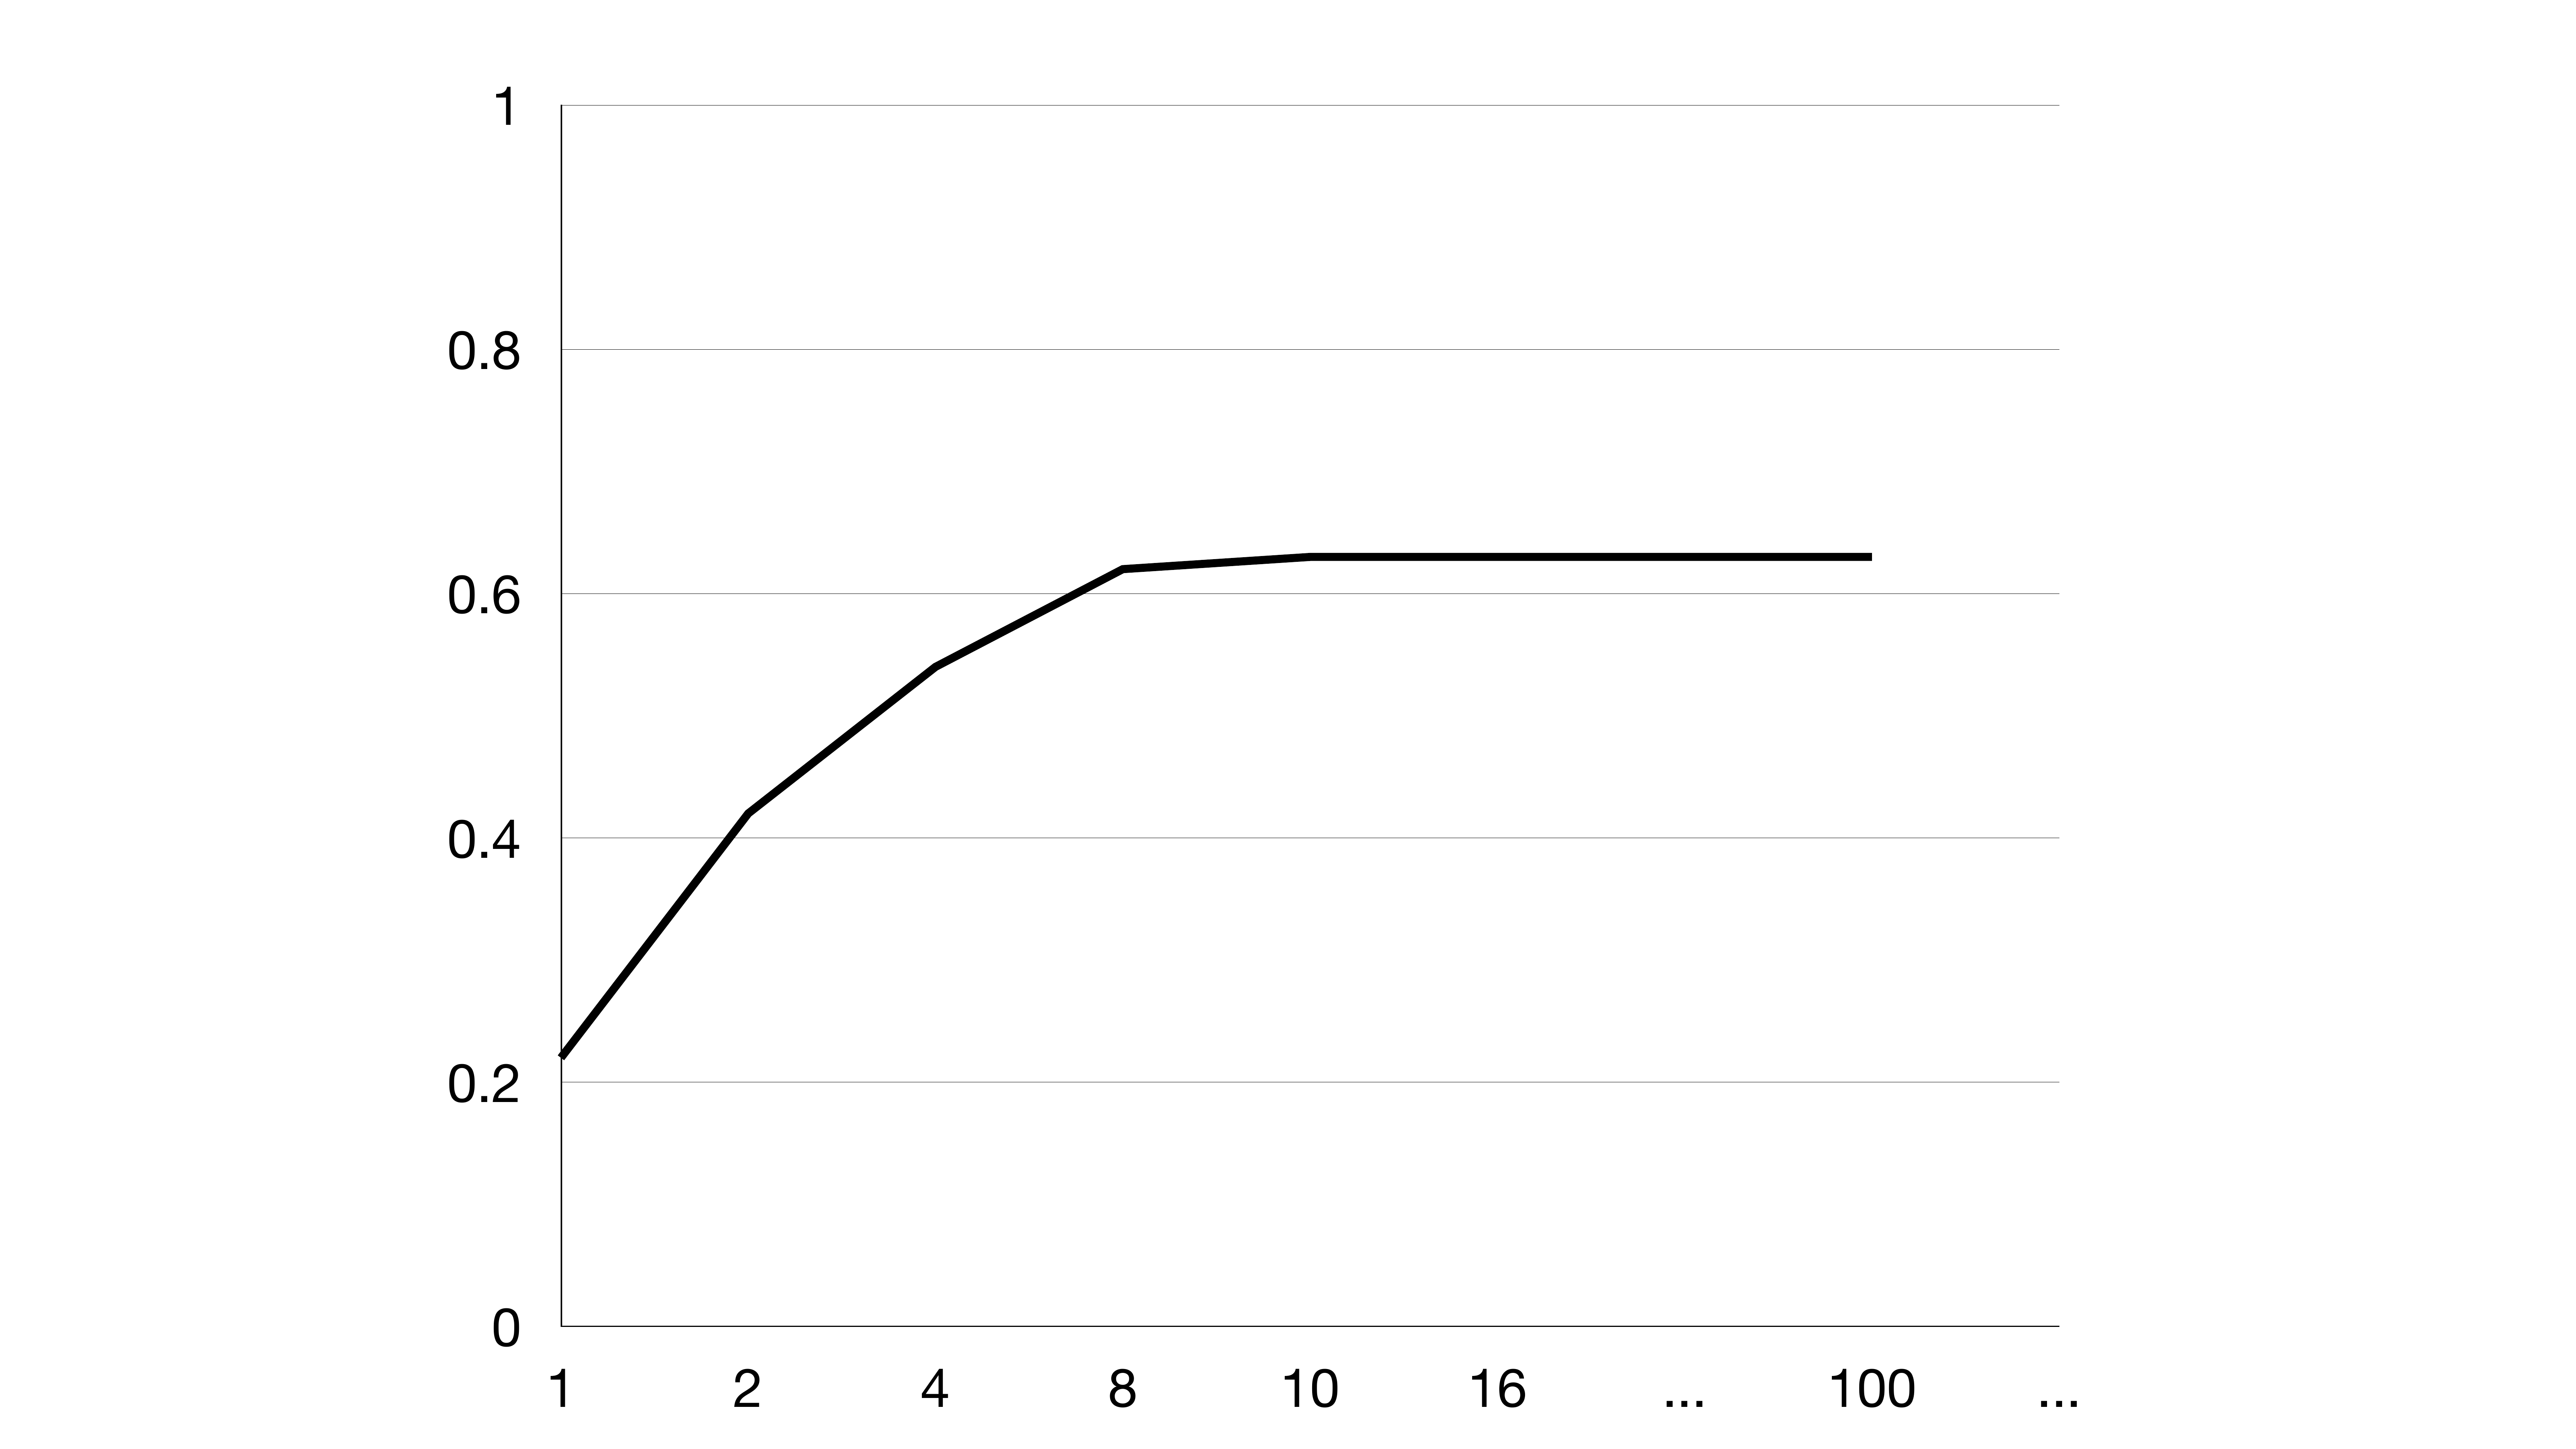}
\caption{CriticGuide results of BART-Large-MNLI score with varying the subset size. Main experiments use 10.}
\label{fig:AppenA}
\end{figure}

\noindent This experiments show the trade-off between computational efficiency and Topic control results. Since our methodology is exact computation, there is a rare change in probability by more than three times, so there is almost no difference in performance from vocab size five or higher.

% 우리 방법론은 exact computation이다보니 왠만해서 2배이상 확률변화가 없고 그러다보니 vocab size 5 이상부턴 거의 성능 차이가 없음. 확률 순위 6등부턴 4배를 곱해도 확률 순위 1등을 넘고 뒤집기가 힘들기 때문임.

% 실험결과: (1,0.22), (2,0.42), (4,0.54), (8,0.62), (10 16 100, 0.63)

\section{Detailed computation of exact distribtuion shift}
\label{sec:appendix B}

\begin{equation}
\begin{aligned}
    P(x_t \vert x_{<t}, a) &= \frac{P(x_t, x_{<t}, a)}{P(x_{<t}, a)}\\
    &= \frac{P(a | x_t, x_{<t})P(x_t, x_{<t})}{P(a | x_{<t})P( x_{<t})}\\
    &= \frac{P(a | x_t, x_{<t})P(x_t | x_{<t})P(x_{<t})}{P(a | x_{<t})P( x_{<t})}\\
    &= \frac{P(a | x_t, x_{<t})P(x_t | x_{<t})}{P(a | x_{<t})}\\
    &= \frac{P(a|x_{\le t})}{P(a|x_{<t})} P(x_t|x_{<t}).
\end{aligned}
\end{equation}

% 어떻게보면 참신한 연산이 아니기때문에 넣어야할지 말아야할지 확신이 안듬.
